# Supplementary material for: Fundus-R1: Training a Fundus-Reading MLLM on Public Data
Source: arXiv:2604.08322 source file (2026-11-07)
Supplement: Supplementary file 1 [file 06_supplement.tex]

\maketitle

\appendix

\setcounter{section}{0}
\setcounter{figure}{0}
\setcounter{table}{0}



In the supplementary material, we provide:
\begin{itemize}
\item Tranining and Hyperparameter settings (Sec.~\ref{sec:hyperparameter}).
\item LLM instruction templates used for data construction and model training (Sec.~\ref{sec:instruction}).
\item Additional details of the reasoning-trace construction pipeline (Sec.~\ref{ssec:details}).
\item Additional experimental results (Sec.~\ref{sec:additional_experimental_results}).

\end{itemize}



\section{Training and Hyperparameter Settings}
\label{sec:hyperparameter}

We train all models in bf16 precision on 8$\times$H800 GPUs (80GB) and perform inference on RTX 3090 GPUs. Given our computational budget, we adopt Qwen2.5-VL~\cite{qwen2.5-VL} (3B/7B) as the backbone. To prevent data contamination, we identify and remove train--test overlaps through image-content matching and exclude all test images and metadata from prompt construction and reasoning-trace generation.

Supervised fine-tuning (SFT) is conducted using LLaMA-Factory~\cite{zheng2024llamafactory} for 2 epochs with a learning rate of $3\times10^{-5}$. RLVR is subsequently performed using the verl framework~\cite{sheng2024hybridflow} for 8 epochs with a learning rate of $1\times10^{-6}$. During RLVR, the sampling temperature is set to 1.0, with 4 rollouts generated per prompt. AdamW is used as the optimizer in both stages.

Since answer formats may vary across MLLMs, we use VLMEvalKit~\cite{duan2024vlmevalkit} for unified answer extraction, ensuring consistent and fair evaluation. The complete hyperparameter configurations for the SFT and RLVR stages are summarized in Tab.~\ref{tab:sft_hyperparams} and Tab.~\ref{tab:rlvr_hyperparams}, respectively. 

\input{tables/SFThyper}
\input{tables/RLVRhyper}


\section{LLM Instruction Templates}
\label{sec:instruction}

This section summarizes the LLM instruction templates used throughout our pipeline, including those for reasoning-trace construction, quality control, and model training.
\input{tables/Prompt}


\section{Details for Data construction}
\label{ssec:details}
This section provides additional details of our reasoning traces, including examples of modality-conditioned domain knowledge and the data cleaning procedures used to improve trace quality.

\subsection{Datasets}
\Cref{tab:datasets} summarizes all training datasets used in our study.
\input{tables/trainingdata}


\subsection{DK-to-VF vocabulary construction.}
We first normalize modality names into a unified abbreviation space to reduce surface variation across data sources. We then parse each DK record into structured knowledge items and process them independently. For each item, we determine whether it expresses affirmative or negated evidence, since negative cues such as \textit{no evidence of} and \textit{absence of} may still correspond to clinically meaningful findings that should be preserved in the vocabulary. Next, we extract lesion-level or sign-level candidate phrases that are visually verifiable under the given modality, while discarding expressions that are non-visual, procedural, or overly abstract. The extracted candidates are further normalized through surface cleanup, stopword filtering, and synonym consolidation, so that semantically equivalent expressions are mapped to the same canonical VF term. Finally, we merge the findings extracted from both the \texttt{required} and \texttt{supportive} fields and remove duplicates to obtain the final $Vocab[y,m]$.

% The complete rule set is summarized in Tab.~\ref{tab:dk2vf_rules}. Tab.~\ref{tab:stopwords} further present the fallback modality mapping and the stopword set used in our implementation.




% \begin{table}[!t]
% \centering
% \small
% \setlength{\tabcolsep}{4pt}
% \renewcommand{\arraystretch}{1.0}

% \begin{tabularx}{\columnwidth}{
%     >{\raggedright\arraybackslash}p{0.30\columnwidth}
%     >{\raggedright\arraybackslash}X
% }
% \toprule
% \textbf{Category} & \textbf{Stopwords} \\
% \midrule
% Articles and determiners 
% & \textit{the, a, an, this, that, these, those} \\

% Prepositions and conjunctions 
% & \textit{of, and, or, with, without, in, on, at, to, for, from, by, as} \\

% Relative and interrogative words 
% & \textit{when, where, which} \\

% Procedural and reporting words 
% & \textit{used, using, indicating, suggesting, indicate} \\

% Generic modifiers 
% & \textit{especially, around, typical, more, advanced, rather, only, primarily} \\

% Generic clinical nouns 
% & \textit{disease, finding, findings, evidence, presence, modality, photograph} \\

% Relational descriptors 
% & \textit{associated, consistent, based} \\

% Auxiliary and weak-content words 
% & \textit{can, may, be, is, are, itself} \\

% Knowledge-structure markers 
% & \textit{supportive, primary} \\
% \bottomrule
% \end{tabularx}
% \caption{Complete stopword list used in DK-to-VF.}
% \label{tab:stopwords}
% \end{table}

Tab.~\ref{tab:dk_vf_examples} presents representative examples of the label- and modality-conditioned domain knowledge used in our pipeline.
\input{tables/dkexample}

\subsection{Data Cleaning Details}

\begin{table*}[!htbp]
\centering
\small
\setlength{\tabcolsep}{4pt}
\renewcommand{\arraystretch}{1.0}

\begin{tabularx}{\textwidth}{
    >{\raggedright\arraybackslash}p{0.08\textwidth}
    >{\raggedright\arraybackslash}p{0.20\textwidth}
    >{\raggedright\arraybackslash}X
    >{\raggedright\arraybackslash}p{0.30\textwidth}
}
\toprule
\textbf{Rule} & \textbf{Operation} & \textbf{Description} & \textbf{Example} \\
\midrule

R1 & Modality normalization 
& Normalize long-form modality names into canonical abbreviations using a predefined fallback mapping.
& \textit{Color fundus photography} $\rightarrow$ \textit{CFP}; \textit{Optical coherence tomography} $\rightarrow$ \textit{OCT} \\

R2 & Knowledge field parsing
& Parse DK into structured fields, e.g., \texttt{required} and \texttt{supportive}, and process each textual item independently.
& \texttt{required: [multiple microaneurysms, dot-blot intraretinal hemorrhages]} \\

R3 & Negative cue detection
& Detect negation using a predefined set of negative cues. If a knowledge item contains a negation pattern, mark it as negative evidence while still extracting the underlying finding term.
& \textit{no evidence of neovascularization} $\rightarrow$ negative cue = \textit{no evidence of}, finding = \textit{neovascularization} \\

R4 & Candidate finding extraction
& Extract visually verifiable lesion- or sign-level noun phrases from each DK item, while discarding non-visual or overly abstract phrases.
& \textit{multiple microaneurysms} $\rightarrow$ \textit{microaneurysm}; \textit{dot-blot intraretinal hemorrhages} $\rightarrow$ \textit{retinal hemorrhage} \\

R5 & Surface cleanup
& Normalize case, remove redundant modifiers, strip punctuation, and singularize plural forms when needed.
& \textit{multiple microaneurysms} $\rightarrow$ \textit{microaneurysm}; \textit{hard exudates} $\rightarrow$ \textit{hard exudate} \\

R6 & Stopword filtering
& Remove high-frequency functional or non-informative words using a predefined stopword list.
& \textit{evidence of hard exudates in the macular region} $\rightarrow$ \textit{hard exudates macular region} \\

R7 & Synonym consolidation
& Map lexical variants and semantically equivalent expressions to a canonical VF form.
& \textit{dot-blot intraretinal hemorrhage}, \textit{retinal hemorrhage} $\rightarrow$ \textit{retinal hemorrhage} \\

R8 & Vocabulary aggregation
& Merge findings extracted from both \texttt{required} and \texttt{supportive} DK items to form the final VF vocabulary for a given label--modality pair.
& \texttt{required} $\cup$ \texttt{supportive} $\rightarrow$ \{\textit{microaneurysm, retinal hemorrhage, hard exudate, cotton-wool spot, neovascularization}\} \\

R9 & De-duplication
& Remove duplicate entries after normalization and preserve only unique canonical VF terms.
& \textit{microaneurysm}, \textit{microaneurysms} $\rightarrow$ \textit{microaneurysm} \\

\bottomrule
\end{tabularx}
\caption{Rule set for converting diagnostic knowledge (DK) into a visual finding (VF) vocabulary.}
\label{tab:dk2vf_rules}
\end{table*}
Before constructing the training data, we perform image-level deduplication across all training datasets to remove duplicated or highly overlapping images. We then apply a coarse-to-fine pipeline to clean the synthesized reasoning traces. The pipeline consists of four stages: format validation, answer consistency checking, rule-based filtering, and LLM-based quality control.

\paragraph{Format validation.}
We verify that the reasoning trace and final answer are enclosed by \texttt{<think>...</think>} and \texttt{<answer>...</answer>}, respectively. Samples with missing, empty, duplicated, malformed, incorrectly ordered, or improperly nested fields are discarded.
\input{tables/compare_with_other_models}
\paragraph{Answer consistency checking.}
We retain only samples whose generated answers exactly match the target labels $y$ used for trace construction.

\paragraph{Rule-based filtering.}
We use regular-expression and heuristic rules to remove traces with repetition, boilerplate text, malformed enumerations, insufficient diagnostic content, or modality--evidence mismatches. For example, an OCT trace is considered suspicious if it relies primarily on unsupported CFP-specific findings.

\paragraph{LLM-based quality control.}
Finally, we use $\mathcal{L}$ to verify each trace against its visual findings $VF[I]$ and modality-conditioned domain knowledge $DK[y,m]$. The verifier assesses modality consistency, coverage of relevant visual findings, validity of the supporting evidence, and consistency with $DK[y,m]$. Using the instruction template in \cref{lst:qc}, it outputs a binary decision. A trace is retained only if it passes all stages and is judged complete, grounded, and consistent.

We use the instruction template provided in \cref{lst:qc}. The verifier outputs a binary decision, and a trace is retained only if it passes all preceding stages and is judged complete, grounded, and consistent.



\subsection{Cost of trace generation}
We use a locally deployed Qwen2.5-VL-32B for VF extraction, and Qwen3-Max API service for trace composition and trace quality check. On average, the online calls take approximately 7.1 seconds and 725 tokens per trace.
The two Qwen models are used only for offline trace generation.



\section{Additional Experimental Results}
\label{sec:additional_experimental_results}

\subsection{Comparison with Existing Models}

\cref{tab:main_arch_perf} further summarizes the vision encoder, LLM backbone, and post-training data used by each MLLM.

\input{tables/purevision}

\cref{tab:purevision} extends the comparison in the main paper by including a broader set of MLLMs.
To examine whether multimodal large language models offer a genuine advantage for fundus image recognition, we compare \model against a broad range of MLLMs, together with strong vision-only models on the FunBench classification tasks. For a controlled comparison, RETFound~\cite{zhou2023foundation}, DERETFound~\cite{sun2025dataefficient}, and DINOv2~\cite{oquab2024dinov2} are equipped with linear classification heads trained on the same task-specific data.

\model consistently outperforms both the MLLM and vision-only baselines. By contrast, existing general-purpose and medical MLLMs do not consistently outperform vision-only models in lesion and disease recognition, and many perform substantially worse than DINOv2-B. These results show that introducing a language model does not inherently improve fundus image recognition. They also highlight a limitation of prior medical MLLM evaluations, which often omit strong vision-only baselines, making it difficult to determine whether the reported gains arise from multimodal reasoning or simply from stronger visual representations.

\subsection{Reliability of the LLM-as-Judge.}

We assess the reliability of the LLM-as-judge on a balanced set of 100 medically plausible and 100 medically flawed reasoning traces, manually annotated by experts. Both classes are written fluently to reduce reliance on superficial linguistic cues. Given each trace and the domain knowledge associated with its predicted answer, $DK[\hat{y},m]$, Qwen3-Max determines whether the reasoning is medically plausible.

As shown in \cref{tab:llm_judge_reliability}, the judge achieves 79\% accuracy and balanced accuracy, correctly classifying 77 plausible and 81 flawed traces. Cohen's $\kappa$ is 0.58, indicating moderate agreement beyond chance. However, it misclassifies 19\% of flawed traces as plausible and 23\% of plausible traces as flawed, suggesting that it is a useful proxy for expert evaluation.



\begin{table}[!htbp]
\centering
\small
\setlength{\tabcolsep}{9pt}
\begin{tabular}{lcc}
\toprule
& \textbf{Human Plausible} & \textbf{Human Flawed} \\
\midrule
\textbf{LLM Plausible} & 77 & 19 \\
\textbf{LLM Flawed}    & 23 & 81 \\
\bottomrule
\end{tabular}
\caption{Agreement between the LLM judge and human experts on the class-balanced reliability test set.}
\label{tab:llm_judge_reliability}
\end{table}


\subsection{Benefits of the Process Reward}
\cref{fig:training_dynamics} further shows the benefit of the process reward: making the model achieve higher answer rewards with shorter and hence more concise rollouts during RLVR training.
\input{figs/training}











\subsection{Failure Cases}
\label{ssec:fail}


\cref{tab:failure-cases} presents several representative failure cases of \model, including misclassifying wet AMD as a more generic CNV pattern, interpreting image blur as cataract, and confusing diabetic retinopathy with retinal vein occlusion. We attribute these errors to two main factors.
\input{figs/fail}
First, the model may map non-specific visual cues directly to familiar disease prototypes without verifying discriminative evidence. This is partly due to our binary VF representation, which records only lesion presence or absence while omitting severity, extent, spatial distribution, and co-occurrence patterns, thereby limiting its ability to distinguish clinically similar diseases.

Second, the DK-guided process reward may favor medically plausible but weakly image-grounded reasoning, especially in the incorrect branch. Because knowledge-consistent explanations can still receive partial credit despite an incorrect prediction, the model may learn to produce fluent, disease-typical descriptions even when the supporting visual evidence is insufficient.





% \input{tables/supplytrace}
% \subsection{Webpages.}


% Tab. provides qualitative examples showcasing our reasoning traces.

% The webpages used in our domain knowledge acquisition pipeline are grouped by source and summarized in Tables~\ref{tab:domain_knowledge_eyewiki}, \ref{tab:domain_knowledge_eyenet}, and~\ref{tab:domain_knowledge_pmc}.
% \input{tables/dfrf}
